# Supplementary material for: Loschmidt-amplitude wave function spectroscopy and the physics of dynamically driven phase transitions
Source: arXiv:1809.00733 source file (2020-02-16)
Supplement: Supplementary file 1 [file SM.pdf]

# Supplementary Information: Loschmidt-amplitude wave function spectroscopy and the physics of dynamically driven phase transitions

D.M. Kennes,<sup>1,2</sup> C. Karrasch,<sup>3,4</sup> and A.J. Millis<sup>5,6</sup>

<sup>1</sup>*Institut für Theorie der Statistischen Physik, RWTH Aachen University and JARA-Fundamentals of Future Information Technology, 52056 Aachen, Germany*

<sup>2</sup>*Max Planck Institute for the Structure and Dynamics of Matter, Center for Free Electron Laser Science, 22761 Hamburg, Germany*

<sup>3</sup>*Dahlem Center for Complex Quantum Systems and Fachbereich Physik, Freie Universität Berlin, 14195 Berlin, Germany*

<sup>4</sup>*Technische Universität Braunschweig, Institut für Mathematische Physik, Mendelssohnstraße 3, 38106 Braunschweig, Germany*

<sup>5</sup>*Department of Physics, Columbia University, 538 West 120th Street, New York, NY 10027 USA*

<sup>6</sup>*Center for Computational Quantum Physics, Flatiron Institute, 162 5th Avenue, New York, NY 10010 USA*

(Dated: February 4, 2020)

---

## RAMP PROFILE

Here we give the equation describing the time dependent profile of  $g(t)$  used in the main text

$$g(t) = \begin{cases} vt & t \in (0, g_{\text{end}}/v] \\ g_{\text{end}} & t \in (g_{\text{end}}/v, g_{\text{end}}/v + t_{\text{wait}}] \\ 2g_{\text{end}} - v(t - t_{\text{wait}}) & t \in (g_{\text{end}}/v + t_{\text{wait}}, 2g_{\text{end}}/v + t_{\text{wait}}) \end{cases}. \quad (1)$$

This ‘double ramp’ is also depicted in the inset to Fig. 1 of the main text.

## DMRG

At time  $t = 0$ , we prepare one of the ferromagnetic ground states of the model, which for  $g(t = 0) = 0$  can be done analytically. We then employ a real time evolution algorithm (see Sect. 7 of Ref. 1) to determine  $|\Psi(t^*)\rangle$  via a propagation from  $t = 0$  to  $t = t^*$  with the time-dependent Hamiltonian  $H(t)$ ; subsequently,  $e^{i(H(t^*) - E_0)t'} |\Psi(t^*)\rangle$  is calculated as a function of  $t'$  using a time-independent  $H(t^*)$ . We employ a fourth-order Suzuki-Trotter decomposition with  $J\Delta t = 0.02$  chosen small enough to give converged results [2]. The numerical cost of this method scales in an exponential fashion with the entanglement in the system. The control parameter encoding the entanglement growth (and with it numerical cost) is the so-called bond-dimension. In our simulations the bond dimension is dynamically increased during the real time evolution such that we obtain numerically exact result. For slow ramps the entanglement growth is slow allowing us to perform simulations up to very large times, before the bond-dimension becomes excessively large.

Additionally, we can obtain a trivial factor of two in the achievable time scale [3] for  $t_{\text{end}}$  by calculating the norm of the state  $|\Psi'\rangle = e^{i(H - E_0)t'/2} |\Psi(t^*)\rangle$  instead of the overlap of  $e^{i(H - E_0)t'} |\Psi(t^*)\rangle$  with  $|\Psi(t^*)\rangle$ .

## FINITE TEMPERATURE GENERALIZATION

It is straightforward to extend the presented ideas to nonzero temperature. Let us assume we have a canonical ensemble

$$\rho = e^{-\beta H} / Z. \quad (2)$$

The generalization of the wavefunction spectrum

$$L(t') = \frac{1}{Z} \text{Tr} \left[ e^{-i(H - E_0)t} \rho \right] = \sum_n e^{-\beta E_n - i(E_n - E_0)t'} \quad (3)$$

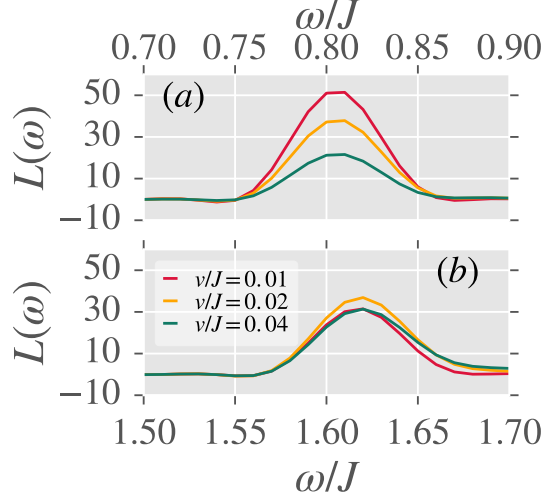

FIG. 1. (a) and (b) Wavefunction spectrum  $L(\omega)$  around frequencies corresponding to  $\Delta$  and  $2\Delta$  for  $g_{\text{end}}/J = 1.4$ ,  $Jt_{\text{wait}} \rightarrow \infty$  and different speeds  $v$ .

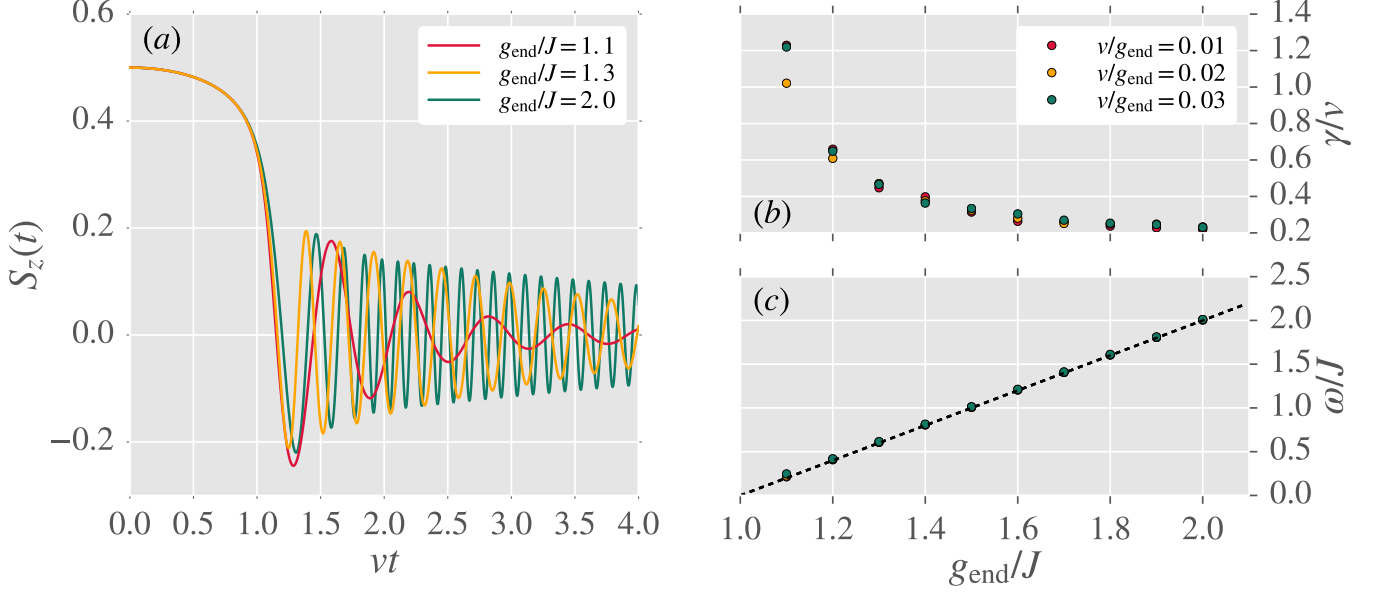

FIG. 2. (a) Dynamics of  $S^z(t)$  for different  $g_{\text{end}}$  and  $v = 0.01g_{\text{end}}$ ,  $t_{\text{wait}} \rightarrow \infty$  and  $N \rightarrow \infty$ . The dynamics at large times fit well to a damped harmonic oscillation  $C \exp(-\gamma t) \sin(\omega t + \delta)$ . (b) and (c) show the fitted parameters  $\gamma$  and  $\omega$  in dependence of  $g_{\text{end}}$ . In (c) the dashed black line is the function  $f(x) = 2|g_{\text{end}} - J|$ .

now yields the Fourier transform

$$L(\omega) = \frac{C}{Z} \sum_n e^{-\beta E_n} \delta(\omega - (E_n - E_0)) \stackrel{E_n \text{ dense}}{=} e^{-\beta w} \rho(w). \quad (4)$$

The  $\beta \rightarrow 0$  limit thus allows to access the state density  $\rho(\omega)$  directly. This is an important quantity and it can, e.g., be used to identify gaps in the many-body spectrum or tell us about the distribution of eigenenergies (as is often used to classify many-body localized systems). The  $\beta > 0$  case allows to analyze where in the spectrum of  $H$  the energy is distributed and allows to analyze how thermal a state looks after, e.g., a quench or ramp by a rigorous comparison of the entire spectrum.

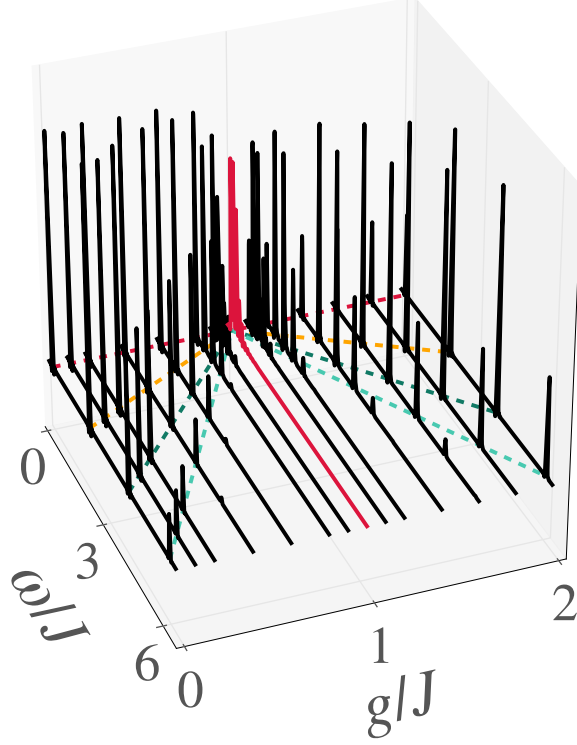

FIG. 3. Wavefunction spectrum  $L(\omega)$  during the second (backward) part of the ramp at times parametrized by  $g(t) = g$  taking the second time  $g(t)$  reaches  $g$ .  $vt_{\text{wait}} = 0.0$  and the other parameters are as in Fig. 5 of the main text. The gap excitation energy  $\omega = 2|g - J|m$  is given as colored dashed lines. The slice for  $g_{\text{stop}} = g_c = 1$  is highlighted in red.

### OBSERVABLES FROM WAVEFUNCTION SPECTROSCOPY

Here we analyze the wave function spectrum in more detail and connect to results obtained by the Kibble-Zurek intuition. We observe that the nonequilibrium probe  $g(t)$  (being spatially uniform) can only create states of total momentum  $k = 0$ . In the one spin-flip sector, the only such state is the minimum energy magnon. In the multi-spin-flip sectors, there is a continuum of states with zero total momentum. However, while present in principle, the ‘multi-magnon continuum’ in practice makes a remarkably small contribution. To see this we present in panels (a) and (b) of Fig. 1 an expanded view of the Loschmidt peaks in the one- and two-spin flip sectors for different ramp speeds. The one-magnon peak is symmetric, with width given solely by the frequency resolution. In the two spin flip sector the fastest ramp shows a weak asymmetry, with slightly more weight on the high energy side; This means that for not too slow ramps a small density of “ $k$  plus  $-k$ ” two-magnon excitations are created, whose density can be controlled by the speed of the ramp.

In order to interpret the magnetization oscillations in terms of these findings, we express  $S^z(t)$  in the eigenstates  $|\{k_j, m_j\}\rangle$  of  $H(t > t_{\text{end}})$ :

$$S^z(t) = \sum_{\{k_j, m_j, m_l, k_l\}} a_{\{k_j, m_j\}}^* a_{\{k_l, m_l\}} e^{i(E_{\{k_j, m_j\}} - E_{\{k_l, m_l\}})t} \langle \{k_j, m_j\} | \sum_i \sigma_i^z | \{k_l, m_l\} \rangle. \quad (5)$$

If a continuum of states were important, then the different terms in the sum would dephase, leading to an exponential

decay of  $S^z(t)$ . However, the Loschmidt analysis shows that the only states that contribute are a small number of zero-momentum states precisely at the bottoms of the few-magnon bands. Therefore, the dominant contribution is the single state that is at the bottom of each  $m$ -magnon band. Including only this contribution we can replace the sum over all  $m$ -magnon states  $\{m\}$  in Eq. (5) by a sum only on the lowest-lying states ( $k = 0$ ), obtaining

$$S^z(t) = \sum_{m,m'} a_{m,k=0} a_{m',k'=0} e^{i(E_{m,k=0} - E_{m',k=0})t} \langle m, k=0 | \sum_i \sigma_i^z | m', k'=0 \rangle \quad (6)$$

We can view the bottom of the magnon band states as quantum defects in the wave function, induced by the ramp. The energy spacings between these are integer multiples of  $2|g_{\text{end}} - J|$  (compare Fig. 2 (b) of the main text). Noting that in the given basis,  $\sigma_i^z$  is the product of sums of raising and lowering operators on adjacent sites and thus connects eigenfunction whose total magnon numbers  $M$  differ by one, this directly explains the oscillations with frequency  $2|g - J|$  depicted in Fig. 1 of the main text. The density of these quantum defects in the ground-state wave function (coherent superposition of higher-excited states) can be read off by determining their density  $\sim |a_m|^2$ , which are the height of the peaks in the wave function spectrum  $L(\omega)$ .

### ESTIMATION OF BEAT FREQUENCY FROM FINITE SIZE

From the frequency difference found in the wave function spectrum at finite  $N$ , we can estimate the first knot in the signal due to the beating in the signal. Taking  $N = 50$  and concentrating only on the three lowest magnon-bands, which captures most of the weight of the wave function after performing a ramp as considered in Fig. 3 of the main text, a knot should appear around times  $\Delta t = t_0 + \pi/(|\Delta E_{\text{magnon}}^1 - \Delta E_{\text{magnon}}^0|)$ , where  $t_0$  has to be estimated somewhere between the time where the ramp crosses the QCP and the time it is completed. In more generic situation where magnons interact a similar estimate should be possible.

### ADDITIONAL DATA FOR $S^z(t)$

The oscillatory dynamics in  $S^z(t)$  are superimposed by a dephasing mechanism which stems from the finite width of the wavefunction spectrum. To disentangle the beating phenomena identified at finite  $N$  in the main text from the dephasing we next concentrate on the dynamics as  $N \rightarrow \infty$ . The wavefunction spectrum would suggest that at  $N \rightarrow \infty$  the differences in energy of the lower  $m$ -magnon bands align perfectly giving rise to a dominant frequency of  $\Omega = 2|g - J|$  in the dynamics of  $S^z$ . The damping of these dynamics at least at  $g$  not too close to 1 via dephasing is given by the width in energy of the  $m$ -magnon peaks themselves, which reduces as the ramp speed is lowered. Indeed all of these prediction from the wavefunction spectrum are confirmed in the dynamics as depicted in Fig. 2. The dephasing is found to scale linearly in  $v$  such that quantum coherence in the wavefunction can be observed on ever larger time scales as the ramp is made slower (compare Fig. 2 (b)).

### WAVEFUNCTION SPECTRUM DURING THE DOUBLE RAMP

Fig. 3 shows the wavefunction spectrum during the time  $t$  of the backward ramp parametrized by  $g(t) = g$  for the second part of the ramp for the same parameters as in Fig. 5 of the main text.

- 
- [1] U. Schollwöck, *Annals of Physics* **326**, 96 (2011), arXiv:1008.3477.
  - [2] D. M. Kennes, *Physical Review B* **96**, 024302 (2017), arXiv:1703.00925.
  - [3] D. M. Kennes and C. Karrasch, *Computer Physics Communications* **200**, 37 (2016), arXiv:1404.3704.
